# Supplementary material for: Data Driven Governing Equations Approximation Using Deep Neural Networks
Source: arXiv:1811.05537 source file (2018-11-13)
Supplement: Supplementary file 1 [file Appendix.tex]

\appendix

\section{Proof of Theorem \ref{thm:main}}
% of \eqref{eq:updatep} and \eqref{eq:updatec}} 
\label{app:derivation}
We start from
the derivation of \eqref{eq:updatec}. By using the orthogonality of the basis $\psi_i$,
the optimization problem \eqref{eq:generalMETHOD} can be rewritten
into the following equivalent problem
\begin{equation}\label{eq:opt:c}
{\bf c}^{(k)} = \mathop{\rm argmin}\limits_{{\bf c} \in {\mathbb{R}}^N}  {\mathcal J}_k({\bf c}),
\end{equation}
where
$$
{\mathcal J}_k({\bf c}) := \big\| {\bf c} - {\bf c}^{(k-1)}   \big\|_2^2 + \frac{1}{\gamma_k}
\left| \langle  {\bf c},{\bf \Psi} ({\bf x}_k) \rangle  -  f_k
\right|^2.
$$
The function
${\mathcal J}_k({\bf c})$ is a convex, because its Hessian matrix is
$2\big({\bf I}+\frac{1}{\gamma_k}{\bf \Psi} ({\bf x}_k) {\bf \Psi}
({\bf x}_k) ^\top \big)$ which is positive definite. 
Thus the problem \eqref{eq:opt:c} is a convex quadratic programming, whose solution is unique and
solves
$$
\frac{\partial {\mathcal J}_k({\bf c}) }{\partial c_j} = 2 \left(  {c}_j - {c}_j^{(k-1)}   + \frac{1}{\gamma_k}
\big( \langle  {\bf c},{\bf \Psi} ({\bf x}_k) \rangle  -  f_k \big) \psi_j ({\bf x}_k) \right)= 0,\quad j=1,2,\cdots,N.
$$
This can be written into vector form
$$
{\bf c} - {\bf c}^{(k-1)} + \frac{1}{\gamma_k} {\bf \Psi} ({\bf x}_k) \big(  {\bf \Psi} ({\bf x}_k)^\top {\bf c}   -  f_k \big) =0,
$$
or,
\begin{equation}\label{eq:der0}
\bigg({\bf I} + \frac{1}{\gamma_k} {\bf \Psi} ({\bf x}_k)   {\bf \Psi} ({\bf x}_k)^\top \bigg){\bf c} = {\bf c}^{(k-1)} + \frac{1}{\gamma_k} f_k {\bf \Psi} ({\bf x}_k).
\end{equation}
Note that the inverse of ${\bf I} + \frac{1}{\gamma_k} {\bf \Psi} ({\bf x}_k)   {\bf \Psi} ({\bf x}_k)^\top$ is
$$
{\bf I} - \frac{1}{ \left\|{\bf \Psi} ({\bf x}_k) \right\|_2^2 + \gamma_k} {\bf \Psi} ({\bf x}_k)   {\bf \Psi} ({\bf x}_k)^\top.
$$
Therefore, we obtain from \eqref{eq:der0} the solution to \eqref{eq:opt:c},
$$
{\bf c}^{(k)} = \bigg( {\bf I} - \frac{1}{ \left\|{\bf \Psi} ({\bf x}_k) \right\|_2^2 + \gamma_k} {\bf \Psi} ({\bf x}_k)   {\bf \Psi} ({\bf x}_k)^\top \bigg)
\bigg( {\bf c}^{(k-1)} + \frac{1}{\gamma_k} f_k {\bf \Psi} ({\bf x}_k) \bigg),
$$
which delivers \eqref{eq:updatec} upon further simplification. The
result of \eqref{eq:updatec} then follows directly from
\eqref{eq:updatep}.

Next, we consider the limiting case of $\gamma_k = 0$ for problem
\eqref{eq:general_0}. Its equivalent form is
\begin{equation}\label{eq:opt:c:g=0}
{\bf c}^{(k)} = \mathop{\rm argmin}\limits_{{\bf c} \in {\mathbb{R}}^N}  \big\| {\bf c} - {\bf c}^{(k-1)}   \big\|_2^2,\quad \mbox{subject~to}~~\langle{\bf c},{\bf \Psi} ({\bf x}_k) \rangle  = f_k.
\end{equation}
Let
$$
{\bf c}^{*}   = {\bf c}^{(k-1)}  + \frac{ f_k -  \langle  {\bf c}^{(k-1)},{\bf \Psi} ({\bf x}_k) \rangle  } { \left\|{\bf \Psi} ({\bf x}_k) \right\|_2^2}   {\bf \Psi} ({\bf x}_k),
$$
then $\langle{\bf c}^*,{\bf \Psi} ({\bf x}_k) \rangle  = f_k$, and
\begin{equation}\label{eq:noname1}
\big\| {\bf c} - {\bf c}^{(k-1)}   \big\|_2^2 = \big\| {\bf c} - {\bf c}^{*}   \big\|_2^2 + \big\| {\bf c}^* - {\bf c}^{(k-1)}   \big\|_2^2,
\end{equation}
where the relation
\begin{align*}
\langle {\bf c} - {\bf c}^{*} , {\bf c}^* - {\bf c}^{(k-1)}  \rangle &= \frac{ f_k -  \langle  {\bf c}^{(k-1)},{\bf \Psi} ({\bf x}_k) \rangle  } { \left\|{\bf \Psi} ({\bf x}_k) \right\|_2^2} \langle {\bf c} - {\bf c}^{*} , {\bf \Psi} ({\bf x}_k) \rangle \\
&=  \frac{ f_k -  \langle  {\bf c}^{(k-1)},{\bf \Psi} ({\bf x}_k) \rangle  } { \left\|{\bf \Psi} ({\bf x}_k) \right\|_2^2} \big( f_k-f_k \big) =0,
\end{align*}
has been used. It is then clear from Eq. \eqref{eq:noname1}
that ${\bf c}^*$ is the solution to problem \eqref{eq:opt:c:g=0}.

\section{Proof of Lemma \ref{thm:gen:c}} \label{app:gen:c}

To prove Theorem \ref{thm:gen:c}, we first introduce a preliminary result.
For notational convenience and without loss of generality, let us assume ${\bf c}^{(0)}={\bf 0}$.
For  ${\bf c}^{(0)} \neq {\bf 0}$, we only need to consider the problem for approximating $f({\bf x})-\langle {\bf c}^{(0)},{\bf \Psi} ({\bf x}) \rangle $,
and replace ${\bf \hat c}$ by (${\bf \hat c}-{\bf c}^{(0)}$) and ${\bf c}^{(k)}$ by (${\bf c}^{(k)}-{\bf c}^{(0)}$).

\subsection{Preliminary} \label{app:prelim}

At the $k$-th iteration, we introduce the notation $\mathbb{E}_k$ to denote the expectation of the random sample ${\bf x}_k$ and the noise $\epsilon_k$, conditioned upon the previous $(k-1)$ random variables $\{{\bf x}_j\}_{1\le j\le{k-1}}, \{\epsilon_k\}_{1\le j\le{k-1}}$, i.e.
$$
\mathbb{E}_k (\cdot) = \mathbb{E}_{{\bf x}_k,\epsilon_k} ( \cdot |{\bf x}_1,\cdots,{\bf x}_{k-1}, \epsilon_1,\cdots,\epsilon_{k-1} ).
$$

\begin{lemma}
	Assume that ${\bf c}^{(0)}={\bf 0}$. The $k$-th iterative solution of the algorithm \eqref{eq:updatec} satisfies
	\begin{equation}\label{eq:lemma1}
	{\mathbb{E}} ( {\bf c}^{(k)} )
=  {\bf Q}^\top {\bf \hat D}^{(k)} {\bf Q} {\bf {\tilde c} },		
	\end{equation}
where ${\bf{\tilde c}} = \big( \tilde c_1, \tilde c_2,\cdots,\tilde c_N \big)^\top$ with $\tilde c_j = ( f,\psi_j )_{L^2_{\tilde \mu}}$, and
$$
{\bf \hat D}^{(k)} = {\rm diag} \{ \hat d_1^{(k)},\cdots, \hat d_N^{(k)} \},\quad \hat d_i^{(k)} = \frac{1-(1-\lambda_i)^k}{\lambda_i}.
$$
\end{lemma}

\begin{proof}
	By taking expectation on \eqref{eq:updatec} we obtain
	\begin{equation*}%\label{eq:Eck}
	\mathbb{E}_k ({\bf c}^{(k)}) = {\bf c}^{(k-1)} +  {\bf \tilde c}  -   {\bf \Sigma} {\bf c}^{(k-1)} = \left( {\bf I} - {\bf \Sigma} \right)  {\bf c}^{(k-1)} +  {\bf \tilde c},
	\end{equation*}
	which implies
	\begin{align*}
	\mathbb{E} ({\bf c}^{(k)}) = \left( {\bf I} - {\bf \Sigma} \right) \mathbb{E} ({\bf c}^{(k-1)}) + {\bf \tilde c}.
	\end{align*}	
	Upon iteratively using this recursive relation, we then have
	$$
	{\mathbb{E}} ( {\bf c}^{(k)} ) =  \sum_{j=1}^k \left( {\bf I} - {\bf \Sigma} \right)^{j-1} {\bf {\tilde c} },
	$$	
	which further yields \eqref{eq:lemma1} via the eigenvalue decomposition of $\bf \Sigma$.
\end{proof}

\subsection{Proof of Lemma \ref{thm:gen:c}}
We now complete the proof of Lemma \ref{thm:gen:c}.
\begin{proof}
The proof starts from the following equality
\begin{align}\nonumber
&{\mathbb{E}}_k \big(\big\| {\bf c}^{(k)} -\hat {\bf c}\big\|^2_2 \big)   =
{\mathbb{E}}_k \Big( \big\|  {\bf c}^{(k-1)} -  \hat {\bf c} + {\bf c}^{(k)} - {\bf c}^{(k-1)} \big\|^2_2 \Big) \\
& = \big\|  {\bf c}^{(k-1)} -  \hat {\bf c}  \big\|^2_2 + 2 \big( {\bf
  c}^{(k-1)} -  \hat {\bf c}  \big)^\top  {\mathbb{E}}_k \big( {\bf
  c}^{(k)} - {\bf c}^{(k-1)} \big) + {\mathbb{E}}_k \Big( \big\| {\bf
  c}^{(k)} - {\bf c}^{(k-1)}
  \big\|^2_2\Big). \label{eq:proof:startpoint} 
\end{align}
The ${\mathbb{E}}_k \big( {\bf c}^{(k)} - {\bf c}^{(k-1)} \big)$ in the second term can be computed as
\begin{align} \nonumber
	{\mathbb{E}}_k \big( {\bf c}^{(k)} - {\bf c}^{(k-1)} \big)
	%= \frac{1}{N_*} \int_D \Big( f({\bf x}) - \langle {\bf c}^{(k-1)}, {\bf\Psi}({\bf x}) \rangle  \Big) {\bf\Psi}({\bf x}) d \tilde \mu \\
	& = \int_D \Big( f({\bf x}) - {\cal P}_V f ({\bf x}) - \langle
          {\bf c}^{(k-1)} - \hat {\bf c}, {\bf\Psi}({\bf x}) \rangle
          \Big) {\bf\Psi}({\bf x}) d \tilde \mu 
	\\
	& =  {\bf e} - {\bf \Sigma} \big( {\bf c}^{(k-1)} - \hat {\bf c} \big), \label{eq:proofwkl1}
\end{align}
and the last term can be expressed as
\begin{align} \nonumber
& {\mathbb{E}}_k \Big(\big\| {\bf c}^{(k)} - {\bf c}^{(k-1)} \big\|^2_2 \Big) =  \int_D  {\mathbb{E}}_{\epsilon_k} \Big( f({\bf x}) + \epsilon_k - \langle {\bf c}^{(k-1)}, {\bf\Psi}({\bf x}) \rangle \Big)^2  d \tilde \omega \\ \nonumber
&  =
\int_D   \Big( f({\bf x}) - {\cal P}_V f ({\bf x}) - \langle {\bf c}^{(k-1)} - \hat {\bf c}, {\bf\Psi}({\bf x}) \rangle  \Big)^2 d \tilde \omega
+ { \|\sigma\|_{L^2_{\tilde \omega}}^2 }
\\
%&  = \frac{1}{N_*}
%\Big( \| f - {\cal P}_V f \|_{L^2_{\tilde{\omega}}}^2 - 2 \tilde{\bf{e}}^\top \big( {\bf c}^{(k-1)} -{\bf \hat c} \big)+  \big( {\bf c}^{(k-1)} -{\bf \hat c} \big)^\top \widetilde{\bf \Sigma} \big( {\bf c}^{(k-1)} -{\bf \hat c} \big)  \Big)
%+ \frac{ \|\sigma\|_{L^2_{\tilde \omega}}^2 }{N_*} \\
&
= {\cal E}+
  \big( {\bf c}^{(k-1)} -{\bf \hat c} \big)^\top \widetilde{\bf \Sigma} \big( {\bf c}^{(k-1)} -{\bf \hat c} \big)
- 2 \tilde {\bf{e}}^\top \big( {\bf c}^{(k-1)} -{\bf \hat c} \big), \label{eq:proofwkl2}
\end{align}
where $\widetilde{\bf \Sigma} := \big( ( \psi_i,\psi_j )_{L^2_{\tilde{\omega}}} \big)_{N \times N}=2{\bf \Sigma}-{\bf \Sigma}_*,$ and $
\tilde {\bf e} := \big(\tilde e_1,\tilde e_2,\cdots,\tilde e_N
\big)^\top={\bf e}-{\bf e}_*$ with $\tilde e_j = ( f-{\cal P}_V f,
\psi_j )_{L^2_{\tilde \omega}}$. 

By substituting \eqref{eq:proofwkl1} and \eqref{eq:proofwkl2} into
\eqref{eq:proof:startpoint}, we then obtain
\begin{align} \nonumber
& {\mathbb{E}}_k \big(\big\| {\bf c}^{(k)} -\hat {\bf c}\big\|^2_2 \big)
\\
% =\big\|  {\bf c}^{(k-1)} -  \hat {\bf c}  \big\|^2_2 +
%\frac{2}{N_*} \Big( {\bf e} - {\bf \Sigma} \big( {\bf c}^{(k-1)} - \hat {\bf c} \big)  \Big)^\top \big( {\bf c}^{(k-1)} -  \hat {\bf c}  \big)
%\\
%&\qquad \quad + \frac{1}{N_*}
%\Big(   \big( {\bf c}^{(k-1)} -{\bf \hat c} \big)^\top \widetilde{\bf \Sigma} \big( {\bf c}^{(k-1)} -{\bf \hat c} %\big)
%- 2 \tilde {\bf{e}}^\top \big( {\bf c}^{(k-1)} -{\bf \hat c} \big) \Big)+{\cal E}\\
& = \big( {\bf c}^{(k-1)} -{\bf \hat c} \big)^\top \big( {\bf I} -  {\bf \Sigma}_*    \big)  \big( {\bf c}^{(k-1)} -{\bf \hat c} \big) + 2 {\bf e}_*^\top \big( {\bf c}^{(k-1)} -{\bf \hat c} \big) + {\cal E} \label{eq:wklproof3}
\\
& \le \big(1- {{ \lambda}_{\min}^*} \big) \| {\bf c}^{(k-1)} -{\bf \hat c} \|_2^2 + 2  {\bf e}_*^\top \big( {\bf c}^{(k-1)} -{\bf \hat c} \big) + {\cal E}. \nonumber
\end{align}
It follows that
\begin{align*}
{\mathbb{E}} \big(\big\| {\bf c}^{(k)} -\hat {\bf c}\big\|^2_2 \big)
& \le \big(1- { \lambda}_{\min}^* \big) {\mathbb{E}} \big(\big\| {\bf c}^{(k-1)} -\hat {\bf c}\big\|^2_2 \big) + 2  {\bf e}_*^\top \big( {\mathbb{E}} ( {\bf c}^{(k-1)} ) -{\bf \hat c} \big) + {\cal E}\\
& =:  r_u {\mathbb{E}} \big(\big\| {\bf c}^{(k-1)} -\hat {\bf c}\big\|^2_2 \big) + {\cal G}_{k-1},
\end{align*}
where
$$
{\cal G}_{k-1} = 2 {\bf e}_*^\top \big( {\bf Q}^\top {\bf \hat D}^{(k-1)} {\bf Q} {\bf {\tilde c} } -{\bf \hat c} \big) + {\cal E},
$$
and \eqref{eq:lemma1} has been used. Repeating the same operation $(k-1)$ times gives
$$
{\mathbb{E}} \big(\big\| {\bf c}^{(k)} -\hat {\bf c}\big\|^2_2 \big)  \le \big\| \hat {\bf c}\big\|^2_2 r_u^k
+ \sum_{j=0}^{k-1}  {\cal G}_j r_u^{k-j-1},
$$
where the last term can be computed as
\begin{align*}
\sum_{j=0}^{k-1}  {\cal G}_j r_u^{k-j-1} & =
2  {\bf e}_*^\top {\bf Q}^\top \bigg( \sum_{j=0}^{k-1}  {\bf \hat D}^{(j)} r_u^{k-j-1} \bigg) {\bf Q} {\bf {\tilde c} }
+
\big( {\cal E} - 2{\bf e}_*^\top {\bf \hat c} \big) \sum_{j=0}^{k-1}  r_u^{k-j-1}
\\
& =
2  {\bf e}_*^\top  \bigg( {\bf Q}^\top {\bf D}^{(k)}  (r_u){\bf Q} {\bf {\tilde c} }  +  \frac{1-r_u^k}{1-r_u} {\bf \Sigma}^{-1} {\bf \tilde c} \bigg)
+
\big( {\cal E} - 2{\bf e}_*^\top {\bf \hat c} \big) \frac{1-r_u^k}{1-r_u}
\\
& =
2  {\bf e}_*^\top  \bigg( {\bf Q}^\top {\bf D}^{(k)} (r_u) {\bf Q} {\bf {\tilde c} }  +  \frac{1-r_u^k}{1-r_u}
\big( {\bf \Sigma}^{-1} {\bf \tilde c} - {\bf \hat c} \big) \bigg)
+ \frac{1-r_u^k}{\lambda_{\min}^*}{\cal E}\\
&
= {\cal B}(r_u) + \frac{1-r_u^k}{\lambda_{\min}^*}{\cal E}.
\end{align*}
Here ${\bf \tilde c}={\bf \Sigma} {\bf \hat c} + {\bf e} $ has been used in the last equality. This completes the proof of the upper bound. Similarly, one can obtain the lower bound.
\end{proof}

\section{Proof of Theorem \ref{thm:gen:tau}} \label{app:2}

\begin{proof}
The proof also starts from \eqref{eq:proof:startpoint}, where the last
term is estimated as
\begin{align*}
& {\mathbb{E}}_k \Big(\big\| {\bf c}^{(k)} - {\bf c}^{(k-1)} \big\|^2_2 \Big) = \int_D  {\mathbb{E}}_{\epsilon_k} \Big( f({\bf x}) + \epsilon_k - \langle {\bf c}^{(k-1)}, {\bf\Psi}({\bf x}) \rangle \Big)^2 \frac{ \left\|{\bf \Psi} ({\bf x}) \right\|_2^2  }{ \left\|{\bf \Psi} ({\bf x}) \right\|_2^2 + \tau } d \tilde \mu \\
& \quad \le
\int_D   \Big( f({\bf x}) - {\cal P}_V f ({\bf x}) - \langle {\bf c}^{(k-1)} - \hat {\bf c}, {\bf\Psi}({\bf x}) \rangle  \Big)^2 d \tilde \mu
+  \| \sigma \|_{L^2_{\tilde \omega}}^2
\\
& \quad =  {\cal E}_0 +
  \big( {\bf c}^{(k-1)} -{\bf \hat c} \big)^\top {\bf \Sigma} \big( {\bf c}^{(k-1)} -{\bf \hat c} \big)
- 2 {\bf{e}}^\top \big( {\bf c}^{(k-1)} -{\bf \hat c} \big) ,
\end{align*}
with $
{\cal E}_0 :=
 \| f - {\cal P}_V f \|_{L^2_{\tilde{\mu}}}^2 + \| \sigma
 \|_{L^2_{\tilde \omega}}^2$.

Hence, we have
\begin{align*}
{\mathbb{E}}_k \big(\big\| {\bf c}^{(k)} -\hat {\bf c}\big\|^2_2 \big)  &
=     \big( {\bf c}^{(k-1)} -{\bf \hat c} \big)^\top
\left( {\bf I} - {\bf \Sigma} \right) \big( {\bf c}^{(k-1)} -{\bf \hat c} \big) +  {\cal E}_0 \\
& \le  \left( 1- \lambda_{\min}\right) \big\| {\bf c}^{(k-1)} -\hat {\bf c}\big\|^2_2 +  {\cal E}_0.
\end{align*}
It follows that
\begin{align*}
{\mathbb{E}} \big(\big\| {\bf c}^{(k)} -\hat {\bf c}\big\|^2_2 \big)
 \le  \left( 1- \lambda_{\min} \right) {\mathbb{E}} \big(\big\| {\bf c}^{(k-1)} -\hat {\bf c}\big\|^2_2 \big)+ {\cal E}_0.
\end{align*}
The proof is completed after repeating the same operation $(k-1)$ times.
\end{proof}

\section{Proof of Theorem \ref{thm:opt:tau}} \label{app:3}

\begin{proof}
	Under the assumption, $d \tilde \mu = \frac{d
          \omega}{N+\tau}$, and ${\bf e}={\bf 0}$, ${\bf \Sigma}=
        \frac{1}{N+\tau} {\bf I}$, the proof also starts from
        \eqref{eq:proof:startpoint}, with the last term estimated as
\begin{align*}
& {\mathbb{E}}_k \Big(\big\| {\bf c}^{(k)} - {\bf c}^{(k-1)} \big\|^2_2 \Big) = \frac{1}{N+\tau} \int_D  {\mathbb{E}}_\epsilon \Big( f({\bf x}) + \epsilon_k - \langle {\bf c}^{(k-1)}, {\bf\Psi}({\bf x}) \rangle \Big)^2 \frac{ \left\|{\bf \Psi} ({\bf x}) \right\|_2^2  }{ \left\|{\bf \Psi} ({\bf x}) \right\|_2^2 + \tau } d \omega \\
&\quad \le  \frac{ \Psi_{\rm sup} }{ (N+\tau)(\Psi_{\rm sup} + \tau)}
\Big( \| f-{\cal P}_{V} f \|_{L^2_\omega}^2  + \|   {\bf c}^{(k-1)} - {\bf{\hat c}} \|_2^2 + \|\sigma \|_{L^2_\omega}^2 \Big) .
\end{align*}
Hence, we have
\begin{align*}
{\mathbb{E}}_k \Big(\big\| {\bf c}^{(k)} -\hat {\bf c}\big\|^2_2\Big)  & \le r_u \big\|  {\bf c}^{(k-1)} -  \hat {\bf c}  \big\|^2_2
+  \frac{ \Psi_{\rm sup} }{ (N+\tau)( \Psi_{\rm sup} + \tau ) }\Big(
 \| f-{\cal P}_{V} f \|_{L^2_\omega}^2 +\| \sigma \|_{L^2_\omega}^2 \Big)  \\
&=: r_u \big\|  {\bf c}^{(k-1)} -  \hat {\bf c}  \big\|^2_2   +   \frac{ \Psi_{\rm sup} {\cal E}_1 }{ (N+\tau)( \Psi_{\rm sup} + \tau)} .
\end{align*}
It follows that
\begin{align*}
{\mathbb{E}} \Big(\big\| {\bf c}^{(k)} -\hat {\bf c}\big\|^2_2\Big) & \le r_u {\mathbb{E}} \Big(\big\|  {\bf c}^{(k-1)} -  \hat {\bf c}  \big\|^2_2 \Big)   + \frac{ \Psi_{\rm sup} {\cal E}_1 }{ (N+\tau)( \Psi_{\rm sup} + \tau)}
\\
& \le \cdots \le r_u^k  \big\|  {\bf c}^{(0)} - \hat {\bf c} \big\|^2_2  + \frac{ \Psi_{\rm sup} {\cal E}_1 }{ (N+\tau)( \Psi_{\rm sup} + \tau)}    \sum_{j=0}^{k-1} r_u^{j}
\\
&
 = r_u^k  \big\| {\bf c}^{(0)} - \hat {\bf c} \big\|^2_2  + \eta_u {\cal E}_1 (1-r_u^k).
\end{align*}
Similarly, one can prove the lower bound.
\end{proof}

\section{Proof of Theorem \ref{thm:opt:psi}} \label{app:4}
\begin{proof}
Under the assumption ${\bf e}_*={\bf 0}$, we have ${\bf \Sigma}_*=
\frac{1+2\tau}{N(1+\tau)^2}{\bf I}$ because of $ (1+1/\tau) d \tilde
\nu = (1+\tau) d \tilde \omega = d \tilde \mu   = \frac{d
  \omega}{N(1+\tau)}$. 
By using \eqref{eq:wklproof3} we have
\begin{align*} 
 {\mathbb{E}}_k \big(\big\| {\bf c}^{(k)} -\hat {\bf c}\big\|^2_2 \big)
& = \big( {\bf c}^{(k-1)} -{\bf \hat c} \big)^\top \big( {\bf I} - {\bf \Sigma}_*    \big)  \big( {\bf c}^{(k-1)} -{\bf \hat c} \big) + {\cal E} \\
& = r \big\| {\bf c}^{(k-1)} -\hat {\bf c}\big\|^2_2 + \frac{1}{N(1+\tau)^2} \Big( \| f - {\cal P}_V f \|_{L^2_{\omega}}^2 + \| \sigma \|_{L^2_{ \omega}}^2 \Big).
\end{align*}
It follows that
\begin{align*}
{\mathbb{E}} \big(\big\| {\bf c}^{(k)} -\hat {\bf c}\big\|^2_2 \big)
= r {\mathbb{E}} \big(\big\| {\bf c}^{(k-1)} -\hat {\bf c}\big\|^2_2 \big)  + \frac{1}{N(1+\tau)^2} \Big( \| f - {\cal P}_V f \|_{L^2_{\omega}}^2 + \| \sigma \|_{L^2_{ \omega}}^2 \Big).
\end{align*}
The proof is then completed after iteratively using the recursive relation.
\end{proof}

\section{A general result} \label{app:5}

Theorems \ref{thm:opt:tau}, \ref{thm:opt:psi} and \ref{thm:opt:tau=0} can be regarded as special cases of the following general result.

\begin{theorem}\label{thm:opt:gen}
	Assume $\gamma_k = \gamma({\bf x}_k)$, and the sampling measure is
	$$
	d \mu = \frac{ \|{\bf\Psi}({\bf x}) \|_2^2 + \gamma({\bf x})  }{ N_*  } d {\omega},
	$$
	with $N_* =N+\int_D \gamma({\bf x}) d\omega$, then the $k$-th iterative solution of \eqref{eq:updatec} satisfies
	\begin{equation*}
	{\mathbb{E}} \big(\|{\bf c}^{(k)} -{\bf \hat c}\|^2_2 \big)  \le
	\| {\bf c}^{(0)} - {\bf \hat c} \|_2^2 r_u^k
	+ \eta_u \left( 1 - r_u^k \right) \bigg(  \| f - {\cal P}_{V} f \|_{L^2_\omega} ^2 +
	\|  \sigma \|_{L^2_{\omega}}^2  \bigg) ,
	\end{equation*}
	and
	\begin{equation*}
	{\mathbb{E}} \big(\|{\bf c}^{(k)} -{\bf \hat c}\|^2_2 \big)  \ge
	\| {\bf c}^{(0)} - {\bf \hat c} \|_2^2 r_\ell^k
	+ \eta_\ell \left( 1 - r_\ell^k \right) \bigg(  \| f - {\cal P}_{V} f \|_{L^2_\omega} ^2 +
	\|  \sigma \|_{L^2_{\omega}}^2  \bigg) ,
	\end{equation*}
	where
	\begin{align*}
	&r_u = 1- \frac{ 2-\Psi_u } {N_*}, \qquad \eta_u = \frac{\Psi_u}{2-\Psi_u},
	\\
	&r_\ell = 1- \frac{ 2-\Psi_\ell } {N_*}, \qquad \eta_\ell = \frac{\Psi_\ell}{2-\Psi_\ell},
	\end{align*}
	with
	$$
	\Psi_u  := \mathop{\rm sup}\limits_{{\bf x}\in D} \frac{ \|{\bf\Psi}({\bf x}) \|_2^2 }{\|{\bf\Psi}({\bf x}) \|_2^2+\gamma({\bf x})}, \qquad \Psi_\ell := \mathop{\rm inf}\limits_{{\bf x}\in D} \frac{ \|{\bf\Psi}({\bf x}) \|_2^2 }{\|{\bf\Psi}({\bf x}) \|_2^2+\gamma({\bf x})}.
	$$
	Therefore
	$$
	\eta_\ell \bigg(  \| f - {\cal P}_{V} f \|_{L^2_\omega} ^2 +
	\|  \sigma \|_{L^2_{\omega}}^2  \bigg)\le \mathop {\lim }\limits_{k \to \infty } {\mathbb{E}} \big(\| {\bf c}^{(k)} -{\bf \hat c}\|^2_2 \big)  \le
	\eta_u \bigg(  \| f - {\cal P}_{V} f \|_{L^2_\omega} ^2 +
	\|  \sigma \|_{L^2_{\omega}}^2  \bigg) .
	$$
\end{theorem}

\begin{proof}
	The proof is similar to that of Theorem \ref{thm:opt:tau}.
\end{proof}
